# Supplementary material for: Data-driven control of room temperature and bidirectional EV charging using deep reinforcement learning: simulations and experiments
Source: arXiv:2103.01886 source file (2021-06-17)
Supplement: Supplementary file 1 [file 20_Appendix_old.tex]

\section{Data pre-processing and splitting}

%%%%%%%%%%%%%%%%%%%%%%%%%%%%%%%%%%%%%%%%%%%%%%%%%%%
\subsubsection{Outlier removal}

Before actually fitting the model, we took a look at the data
and discovered an irregularity
in the data as shown in figure \ref{fig:battery_outliers}.
One can see that there are quite a few samples where
the active power applied was very large but the SoC
changed barely. After further investigation, it was found
that the cause of those data points was an experiment
that was conducted with the battery where the control 
inputs where changed with much higher frequency than the
measuring frequency. Therefore, the data in the database
fails to capture these dynamics accurately. Since
we do not intend to control the battery at such a high
frequency, we also removed those data samples from the
dataset, even if there was nothing wrong with the data
collecting mechanism. This was done by identifying the time at which 
the experiments were conducted and removing all the data from
that time afterward.

\begin{figure}
  \centering
  \includegraphics[page=1,width=\columnwidth]{Imgs/Battery/WithOutliers.pdf}
  \caption{Battery charging model with unphysical samples. Shown with
    a linear fit demonstrating the influence of the outliers.}
  \label{fig:battery_outliers}
\end{figure}

\begin{figure}
  \centering
  \includegraphics[page=1,width=\columnwidth]{Imgs/Battery/ResVsSoc.pdf}
  \caption{Residuals plotted versus the SoC in the previous step}
  \label{fig:bat_soc_res}
\end{figure}

\section{PW linear vs. RNN model comparison for the weather model}
To or not to include.If yes then:

- include section: 3.1.3    Motivating RNN usage

- include the first part of the section 3.1.4. on the room model where the difference between partial and full room temperature model (fig 3.6) and the slight difference (<0.2 max abs err) between them. using the "imperfect" weather model compared to using the perfect weather prediction. 

The top plot shows the evaluation of $m^{rtemp}$ that  predicts only the room temperature and no other series. Therefore, in order to assess the performance of the predictions over more than one step, the ground truth of the weather and the water temperatures was used to feed to the model. This is not the case in the bottom plot of Figure 3.6, there the complete model mfull was used. 

It can be observed that the model predicting all series performs only slightly worse than the partial model using the ground truth for the weather and the water temperatures inputs.

It can be seen that the predictions of both models are stable and do not diverge, 
even though there is an unexpected peak after a few days. %Since we are not interested in predictions over more than a day, we do not care about this specic peak happening.


\subsection{Physical inconsistency of the RNN room temperature model}

%%%%%%%%%%%%%%%%%%%%%%%%%%%%%%%%%%%%%%%%%%%%%%%%%%%%
%%%%%%%%%%%%%%%%%%%%%%%%%%%%%%%%%%%%%%%%%%%%%%%%%%%%
\subsection{Separate heating and cooling agents}

First, all together presented:


\begin{figure}
  \centering
  \includegraphics[page=1,width=\columnwidth]{Imgs/RoomRL_R43_T22_26/DetailAnalysis_10000_Const_1.0_Const_0.0_RuleBasedControl_DDPG_NEP500000.pdf}
  \caption{Evaluation of the DDPG reinforcement learning agent}
  \label{fig:heat_cool_eval}
\end{figure}


And then separated. Comment on this.
Discussing the figure on Heating only agent evaluation.
How is it possible that the "valves closed" agent has better comfort bounds than valves open for the heating case? Isn't that a very strange result… Would not you expect that if you don't heat at all that the comfort would be worse than if you heat all the time? Maybe not. Depending on the building. In a building with large windows, this may be the expected behavior that no heating at all is good. The problematic result can be that RBC is actually doing worse in terms of comfort violation than not doing anything (0.55 < 0.57).

You are right, this is a bit a strange behavior.
But also, this plot shows the case with the reference tracking. 
There, it could be explained with overheating of the rule-based agent, since
it heats as long as the temperature is below the threshold, and then it is likely to 
overshoot. But this also suggests that it could be tuned more to become better, 
maybe already stop 0.5 deg C before the reference (22.5 in this case).
Not doing anything is probably also better since the temperature drops very slowly,
the experiments that I did over Christmas showed this also. And further, the episode 
is only 12h, so the temperature will not drop a lot. For this reason, I guess, it is better
than the rule-based agent. 

\begin{figure}
    \centering
    \subfloat[Heating]
            {{\includegraphics[width=\columnwidth]
            {Imgs/RoomRL_R43_T22_26/DetailAnalysis_10000_Const_1.0_Const_0.0_RuleBasedControl_DDPG_NEP500000_Heat.pdf}}}%
    
    \subfloat[Cooling]
            {{\includegraphics[width=\columnwidth]
            {Imgs/RoomRL_R43_T22_26/DetailAnalysis_10000_Const_1.0_Const_0.0_RuleBasedControl_DDPG_NEP500000_Cool.pdf}}}%
    \caption{Separate evaluation of heating (top) and cooling cases (bottom) }%
    \label{fig:cool_heat_separate}%
\end{figure}
